# Supplementary material for: Designing Multi-Stage Coupled Convex Programming with Data-Driven McCormick Envelope Relaxations for Motion Planning
Source: arXiv:2109.06516 source file (2021-09-14)
Supplement: Supplementary file 1 [file sect_appendix.tex]

Since this component is ``controlled" by the loading through static equilibrium (constraint E,F), it cannot take its full $[-1,1]$ range. In Fig. \ref{Fig:notations}, $f_{iz}$ cannot be negative, due to the existence of gravitational load. In the case when the body is flat, we can explicitly solve the 
contact force $f_{iz}$ as a function of body gravity and toe positions. In Fig. \ref{Fig:notations}, $\textbf{f}_{1z}$ can be solved through moment balance (and similar for $\textbf{f}_{2z}$ and $\textbf{f}_{3z}$):

\begin{equation}
    (\textbf{p}_{3}-\textbf{p}_{2})\times(\textbf{p}_{COM}-\textbf{p}_{2}) \cdot \textbf{G} + (\textbf{p}_{3}-\textbf{p}_{2})\times(\textbf{p}_{1}-\textbf{p}_{2}) \cdot \textbf{f}_{1z} =0
    \label{Eqn:moment_balance}
\end{equation}{}

Equation (\ref{Eqn:moment_balance}) demonstrates a complicated dependency on $\textbf{G}$ and $\textbf{p}_{i}$. However, there is no need to directly attack it. The toe positions are subject to workspace constraints. Thus we can retrieve an upper and lower bound of the contact force simply by search over all possible postures. We find two extreme cases to be $\textbf{f}_{iz-min}=\textbf{0}$ and $\textbf{f}_{iz-max}=0.6\textbf{G}$, which gives the bound $f_{iz}\in[0,0.4]$. The original and range limited surfaces are shown in Fig. \ref{Fig:Cutted_bilinear_constraints} on the left. Note that the range $f_{iz}\in[0,0.4]$ exist because of constraint E and F, thus no matter we use the original envelope or shrunken envelope, this range is always imposed. If the original envelope is used, the effective envelope is the green region in Fig. \ref{Fig:2D_envelope}. The shrunken envelope designed here (yellow region in Fig. \ref{Fig:2D_envelope}) cuts down the $m_{ijk}$ range but not $f_{ik}$ range.
